# Supplementary material for: Randomized interventional effects in semicompeting risks, with application to a hematopoietic cell transplantation study
Source: arXiv:2412.06114 source file (2026-05-19)
Supplement: Supplementary file 1 [file Supp.pdf]

# Supplementary Material to "Randomized interventional effects for semicompeting risks, with application to allogeneic stem cell transplantation study"

## A Identification of interventional effects without confounders

The hazard-type draw:

$$
\begin{aligned}
P\{d\tilde{N}_2(t; z_2, G(t; z_1)) = 1\} &= \sum_{n_1 \in \{0,1\}} P\{d\tilde{N}_2(t; z_2, G(t; z_1)) = 1, G(t; z_1) = n_1\} \\
&= \prod_{s \in (0,t)} P\{dG(s; z_1) = 0 \mid G(s^-; z_1) = \tilde{N}_2(s^-; z_2, G(\cdot; z_1)) = 0\} \\
&\qquad P\{d\tilde{N}_2(s; z_2, G(s; z_1)) = 0 \mid G(s; z_1) = \tilde{N}_2(s^-; z_2, G(\cdot; z_1)) = 0\} \\
&\qquad P\{dG(t; z_1) = 0 \mid G(t^-; z_1) = \tilde{N}_2(t^-; z_2, G(\cdot; z_1)) = 0\} \\
&\quad P\{d\tilde{N}_2(t; z_2, G(t; z_1)) = 1 \mid G(t; z_1) = \tilde{N}_2(t^-; z_2, G(\cdot; z_1)) = 0\} \\
&\quad + \int_0^t \prod_{s \in (0,r)} P\{dG(s; z_1) = 0 \mid G(s^-; z_1) = \tilde{N}_2(s^-; z_2, G(\cdot; z_1)) = 0\} \\
&\qquad P\{d\tilde{N}_2(s; z_2, G(s; z_1)) = 0 \mid G(s; z_1) = \tilde{N}_2(s^-; z_2, G(\cdot; z_1)) = 0\} \\
&\qquad P\{dG(r; z_1) = 1 \mid G(r^-; z_1) = \tilde{N}_2(r^-; z_2, G(\cdot; z_1)) = 0\} \\
&\qquad \prod_{s \in [r,t)} P\{d\tilde{N}_2(s; z_2, G(s; z_1)) = 0 \mid \tilde{N}_2(s^-; z_2, G(\cdot; z_1)) = 0, G(s; z_1) = 1\} \\
&\quad P\{d\tilde{N}_2(t; z_2, G(t; z_1)) = 0 \mid \tilde{N}_2(t^-; z_2, G(\cdot; z_1)) = 0, G(t; z_1) = 1\} \\
&= \prod_{s \in (0,t)} \{1 - d\Lambda_0(s; z_2)\}\{1 - d\Lambda_*(s; z_1)\}\{1 - d\Lambda_*(t; z_1)\}\{1 - d\Lambda_0(t; z_2)\} \\
&\quad + \int_0^t \prod_{s \in (0,r)} \{1 - d\Lambda_0(s; z_2)\}\{1 - d\Lambda_*(s; z_1)\} d\Lambda_*(r; z_1) \prod_{s \in [s,t)} \{1 - d\Lambda_1(s; z_2)\} d\Lambda_1(t; z_2) \\
&= \exp\{-\Lambda_0(t; z_2) - \Lambda_*(t; z_1)\} d\Lambda_1(t; z_2) \\
&\quad + \int_0^t \exp\{-\Lambda_0(r; z_2) - \Lambda_*(r; z_1)\} \exp\{-\Lambda_1(t; z_2) + \Lambda_1(s; z_2)\} d\Lambda_*(r; z_1) d\Lambda_1(t; z_2), \\
F_{\mathrm{IE}}(t; z_1, z_2) &= \int_0^t P\{d\tilde{N}_2(s; z_2, G(s; z_1)) = 1\} \\
&= \int_0^t \exp\{-\Lambda_0(s; z_2) - \Lambda_*(s; z_1)\} d\Lambda_0(s; z_2) \\
&\quad + \int_0^t \exp\{-\Lambda_0(s; z_2) - \Lambda_*(s; z_1)\}[1 - \exp\{-\Lambda_1(t; z_2) + \Lambda_1(s; z_2)\}] d\Lambda_*(s; z_1).
\end{aligned}
$$

The prevalence-type draw:

$$
\begin{aligned}
d\Lambda(t; z_1, z_2) :&= P\{d\tilde{N}_2(t; z_2, G(t; z_1)) = 1 \mid \tilde{N}_2(t; z_2, G(\cdot; z_1)) = 0\} \\
&= \sum_{n_1 \in \{0,1\}} P\{G(t; z_1) = n_1 \mid \tilde{N}_2(t^-; z_2, G(\cdot; z_1)) = 0\} \\
&\qquad P\{d\tilde{N}_2(t; z_2, G(t; z_1)) = 1 \mid \tilde{N}_2(t^-; z_2, G(\cdot; z_1)) = 0, G(t; z_1) = n_1\}
\end{aligned}
$$

$$
\begin{aligned}
&= \sum_{n_1 \in \{0,1\}} P\{\tilde{N}(t; z_1) = n_1 \mid \tilde{N}_2(t^-; z_1) = 0\} P\{d\tilde{N}_2(t) = 1 \mid \tilde{N}_2(t^-; z_2) = 0, \tilde{N}_1(t; z_2) = n_1\} \\
&= \sum_{n_1 \in \{0,1\}} w_{n_1}(t; z_1) d\Lambda_{n_1}(t; z_2), \\
P\{d\tilde{N}_2(t; z_2, G(t; z_1)) = 1\} &= \prod_{s \in [0,t)]} P\{d\tilde{N}_2(s; z_2, G(s; z_1)) = 0 \mid \tilde{N}_2(s; z_2, G(\cdot; z_1)) = 0\} \\
&\qquad P\{d\tilde{N}_2(t; z_2, G(t; z_1)) = 1 \mid \tilde{N}_2(t; z_2, G(\cdot; z_1)) = 0\} \\
&= \exp\{-\Lambda(t; z_1, z_2)\} d\Lambda(t; z_1, z_2), \\
F_{\mathrm{IE}}(t; z_1, z_2) &= \int_0^t P\{d\tilde{N}_2(s; z_2, G(s; z_1)) = 1\} \\
&= 1 - \exp\{-\Lambda(t; z_1, z_2)\} \\
&= 1 - \exp\left\{\int_0^t \sum_{n_1 \in \{0,1\}} w_{n_1}(s; z_1) d\Lambda_{n_1}(s; z_2)\right\}.
\end{aligned}
$$

The identifiability of $d\Lambda_{n_1}(t; z_2)$, $d\Lambda_*(t; z_1)$ and $w_{n_1}(t; z_2)$ is shown in Deng et al. (2024b) under Markovness, ignorability, positivity, random censoring and consistency.

# B Direct and indirect effects without confounders

## B.1 Natural effects

Given a fixed counting process of the intermediate event $\tilde{n}(\cdot)$, let $\tilde{N}_2(t; z, \tilde{n}(\cdot)) = \int_0^t d\tilde{N}_2(s; z, \tilde{n}(s))$ be the counterfactual counting process of the terminal event under treatment $z \in \{0, 1\}$. Since the counting process can only jump once from 0 to 1, we can determine the full counting process as long as we know the time it jumps.

To evaluate the direct and indirect effects, it is straightforward to define the treatment effect by contrasting two counterfactual CIFs by appropriately controlling the intermediate event. First, we set the treatment at $z_1$ and obtain a counting process of the intermediate event $\tilde{N}_1(\cdot; z_1)$. Next, we supply this process to the terminal event process, resulting in a counterfactual counting process $\tilde{N}_2(t; z_2, \tilde{N}_1(\cdot; z_1))$ involving cross-world quantities. Let $F_{\mathrm{NE}}(t; z_1, z_2) = P\{\tilde{N}_2(t; z_2, \tilde{N}_1(\cdot; z_1)) = 1\}$ be the counterfactual CIF of the terminal event. The natural direct effect (NDE)

$$
\mathrm{NDE}(t, z_1) = F_{\mathrm{NE}}(t; z_1, 1) - F_{\mathrm{NE}}(t; z_1, 0),
$$

and the natural indirect effect (NIE)

$$
\mathrm{NIE}(t; z_2) = F_{\mathrm{NE}}(t; 1, z_2) - F_{\mathrm{NE}}(t; 0, z_2).
$$

When $z_1 = z_2 = z$, the potential CIF $F(t; z) = F_{\mathrm{NE}}(t; z, z)$. The total effect is the summation of natural direct and indirect effects,

$$
\mathrm{TE}(t) = F(t; 1) - F(t; 0) = \mathrm{NDE}(t; 0) + \mathrm{NIE}(t; 1).
$$

**Remark S1.** *There are two ways to decompose the total effect,* $\mathrm{TE}(t) = \mathrm{NDE}(t; 0) + \mathrm{NIE}(t; 1) = \mathrm{NDE}(t; 1) + \mathrm{NIE}(t; 0)$. *In practice, we usually adopt the first decomposition. Consider an example where the treatment is a novel drug to prevent the terminal event and the control is placebo. To study the direct effect of this drug, we may assume that the risk of the intermediate event is controlled at the level under placebo. However, it is not reasonable to let all individuals take the drug for the intermediate event while taking placebo for the terminal event. In other words, since the drug is to treat the terminal (primary) event, we assume* $z_1 \le z_2$.

The core assumption to identify the natural effects is sequential ignorability. We assume that the cause-specific hazard of the terminal event

$$
\begin{aligned}
d\Lambda_{n_1}(t; z_1, z_2) :&= P\{d\tilde{N}_2(t; z_2, \tilde{N}_1(\cdot; z_1)) = 1 \mid \tilde{N}_2(t^-; z_2, \tilde{N}_1(\cdot; z_1)) = 0, \tilde{N}_1(t; z_1) = n_1\} \\
&= P\{d\tilde{N}_2(t; z_2) = 1 \mid \tilde{N}_2(t^-; z_2) = 0, \tilde{N}_1(t; z_2) = n_1\} = d\Lambda_{n_1}(t; z_2)
\end{aligned} \tag{S1}
$$

does not rely on the treatment associated with the intermediate event $z_1$. This assumption means that the instantaneous risk of encountering the terminal event at time $t$ only depends on the treatment associated with the terminal event $z_2$ and the current

status of the intermediate event $n_1$ as long as the terminal event has not occurred at time $t$. As for the risk of the intermediate event, Deng et al. (2024b) assumed that the cause-specific hazard of the intermediate event

$$\begin{aligned} d\Lambda_*(t; z_1, z_2) :&= P\{d\tilde{N}_1(t; z_1) = 1 \mid \tilde{N}_2(t^-; z_2, \tilde{N}_1(\cdot; z_1)) = 0, \tilde{N}_1(t^-; z_1) = 0\} \\ &= P\{d\tilde{N}_1(t; z_1) = 1 \mid \tilde{N}_2(t^-; z_1) = 0, \tilde{N}_1(t^-; z_1) = 0\} = d\Lambda_*(t; z_1) \end{aligned} \tag{S2}$$

does not rely on the treatment associated with the terminal event $z_2$. Under Assumptions (S1) and (S2), the counterfactual CIF the terminal event

$$\begin{aligned} F_{\mathrm{NE}}(t; z_1, z_2) = &\int_0^t \exp\{-\Lambda_0(s; z_2) - \Lambda_*(s; z_1)\} d\Lambda_0(s; z_2) \\ &+ \int_0^t \exp\{-\Lambda_0(s; z_2) - \Lambda_*(s; z_1)\}[1 - \exp\{-\Lambda_1(t; z_2) + \Lambda_1(s; z_2)\}] d\Lambda_*(s; z_1) \end{aligned} \tag{S3}$$

is identifiable (Deng et al., 2024b). The natural direct effect is interpreted as the difference in counterfactual CIFs of the terminal event by switching the treatment while holding the hazard of the intermediate event unchanged. The natural indirect effect is the difference in counterfactual CIFs by letting the hazard of the intermediate event change with treatment while holding the cause-specific hazards of the terminal event unchanged.

**Remark S2.** *Another approach to control the "risk" of the intermediate event is to control the prevalence. Huang (2021) assumed that the prevalence of the intermediate event in the counterfactual world*

$$\begin{aligned} w_{n_1}(t; z_1, z_2) :&= P\{\tilde{N}_1(t; z_1) = n_1 \mid \tilde{N}_2(t^-; z_2, \tilde{N}_1(\cdot; z_1)) = 0\} \\ &= P\{\tilde{N}_1(t; z_1) = n_1 \mid \tilde{N}_2(t^-; z_1) = 0\} = w_{n_1}(t; z_1) \end{aligned} \tag{S4}$$

*does not rely on the treatment associated with the terminal event $z_2$. Under Assumptions* (S1) *and* (S4)*, the counterfactual CIF of the terminal event*

$$F_{\mathrm{NE}}(t; z_1, z_2) = 1 - \exp\left\{\int_0^t \sum_{n_1 \in \{0,1\}} w_{n_1}(s; z_1) d\Lambda_{n_1}(s; z_2)\right\}. \tag{S5}$$

*It is easy to verify that Equations* (S3) *and* (S5) *are identical when $z_1 = z_2$. The natural direct effect is interpreted as the difference in counterfactual CIFs of the terminal event by switching the treatment while holding the prevalence of the intermediate event unchanged. The natural indirect effect is the difference in counterfactual CIFs of the terminal event by letting the prevalence of the intermediate event change with treatment while holding the cause-specific hazards of the terminal event unchanged.*

We recommend adopting Assumption (S2) rather than (S4) as the sequential ignorability, due to the following two reasons. First, the hazard of the intermediate event is a term in the likelihood, while the prevalence is not. The assumption on counterfactuals should reflect the underlying data generating mechanism. It is well acknowledged that hazards can be modeled by the proportional hazards model, but there are no clear models for the prevalence. It is not intuitive to propose a data generating mechanism with the prevalence of the intermediate event variational independent of the cause-specific hazards of the terminal event. By increasing the cause-specific hazard of the direct terminal event $d\Lambda_0(t; z)$ and holding the cause-specific hazard of the intermediate event-induced terminal event $d\Lambda_1(t; z)$, there will be fewer survivors at the nearest future, and thus the prevalence of the intermediate event $w_1(t; z)$ will increase.

Second, estimation based on the hazard-type assumption is computationally more efficient. We take the nonparametric scenario as an example where there are no confounders. The asymptotic distribution of the prevalence-type CIF estimator involves the asymptotic distribution of the prevalence estimator, which involves high computational burden since we need to calculate a covariance matrix whose dimension is nearly the sample size. In contrast, the asymptotic distribution of hazard-type CIF estimator is the summation of three independent martingales compounded by predictable processes. So we can simply use a cumulative summation algorithm to estimate the asymptotic variance (Deng et al., 2024b).

There are some limitations for the framework of natural effects. First, the sequential ignorability is hard to explain. By definition, $\tilde{N}_1(t; z_1)$ should only be relevant to $z_1$. However, Assumption (S2) indicates that the hazard of $\tilde{N}_1(t; z_1)$ can be influenced by $\tilde{N}_2(t; z_2; \tilde{N}_1(\cdot; z_1))$, which is counterintuitive. This is due to the nature of semicompeting risks, where the statuses of the intermediate and terminal events can influence the at-risk processes of each other. Rigorously speaking, the counterfactual counting process of the intermediate event $\tilde{N}_1(t; z_1) = \int_0^t I\{\tilde{N}_2(s^-; z_2, \tilde{N}_1(\cdot; z_1)) = 0\} d\tilde{N}_1(s; z_1)$ in the counterfactual world. Second, Assumption (S2) basically means that there is no unmeasured confounding between the statuses of intermediate and terminal events, which can easily be violated. In the presence of time-varying confounders, the natural effects are generally not identifiable.

## B.2 Separable effects

An interventionist approach proposes to manipulate the cause-specific hazards, referred to as the separable effects framework (Robins et al., 2022). The treatment $Z$ is assumed to be comprised of two components $(Z_1, Z_2)$, where $Z_1$ influences the hazard of the intermediate event and $Z_2$ influences the cause-specific hazards of the terminal event. In a realized trial, $Z_1 = Z_2$. In the counterfactual world, we can let $Z_1$ and $Z_2$ take different values. The jumps of the intermediate and terminal events at time $t$ can be written as potential outcomes $d\tilde{N}_1(t; z_1, z_2)$ and $d\tilde{N}_2(t; z_1, z_2, n_1)$, respectively, where $(z_1, z_2)$ is the combination of treatment components and $n_1$ is the status of the intermediate event at time $t$. We denote the counterfactual counting processes of the intermediate event and terminal event as $\tilde{N}_1(t; z_1, z_2) = \int_0^t d\tilde{N}_1(t; z_1, z_2)$ and $\tilde{N}_2(t; z_1, z_2) = \int_0^t d\tilde{N}_2(s; z_1, z_2, \tilde{N}_1(s; z_1, z_2))$, respectively. By contrasting the counterfactual CIFs of the terminal event $F_{\text{SE}}(t; z_1, z_2) = P\{\tilde{N}_2(t; z_1, z_2) = 1\}$, the separable direct effect (SDE)

$$\text{SDE}(t; z_1) = F_{\text{SE}}(t; z_1, 1) - F_{\text{SE}}(t; z_1, 0)$$

and the separable indirect effect (SIE)

$$\text{SIE}(t; z_2) = F_{\text{SE}}(t; 1, z_2) - F_{\text{SE}}(t; 0, z_2).$$

Even if there is post-treatment unmeasured confounding, the separable effects have meaningful causal explanation. When $z_1 = z_2 = z$, the potential CIF $F(t; z) = F_{\text{SE}}(t; z, z)$. The total effect is the summation of the separable direct and indirect effects,

$$\text{TE}(t) = F(t; 1) - F(t; 0) = \text{SDE}(t; 0) + \text{SIE}(t; 1).$$

The core assumption for identification is the dismissible components condition,

$$\begin{aligned} d\Lambda_{n_1}(t; z_1, z_2) :&= P\{d\tilde{N}_2(t; z_1, z_2, \tilde{N}_1(t; z_1, z_2)) = 1 \mid \tilde{N}_2(t^-; z_1, z_2) = 0, \tilde{N}_1(t; z_1, z_2) = n_1\} \\ &= P\{d\tilde{N}_2(t; z_2, \tilde{N}_1(t; z_2)) = 1 \mid \tilde{N}_2(t^-; z_2) = 0, \tilde{N}_1(t; z_2) = n_1\} = d\Lambda_{n_1}(t; z_2), \end{aligned} \tag{S6}$$

$$\begin{aligned} d\Lambda_*(t; z_1, z_2) :&= P\{d\tilde{N}_1(t; z_1, z_2) = 1 \mid \tilde{N}_2(t^-; z_1, z_2) = 0, \tilde{N}_1(t^-; z_1, z_2) = 0\} \\ &= P\{d\tilde{N}_1(t; z_1) = 1 \mid \tilde{N}_2(t^-; z_1) = 0, \tilde{N}_1(t^-; z_1) = 0\} = d\Lambda_*(t; z_1). \end{aligned} \tag{S7}$$

The dismissible components condition generally means that there is no unmeasured confounding between the statuses of intermediate and terminal events, similar to sequential ignorability. This assumption is not testable in realized trials, but it provides an opportunity. In future experiments, if we know exactly the components of $Z_1$ and $Z_2$, we may possibly assign different values to $Z_1$ and $Z_2$ and test this assumption. Under Assumptions (S6) and (S7), the counterfactual CIF of the terminal event $F_{\text{SE}}(t; z_1, z_2)$ shares the same identification formula with Equation (S3),

$$\begin{aligned} F_{\text{SE}}(t; z_1, z_2) = &\int_0^t \exp\{-\Lambda_0(s; z_2) - \Lambda_*(s; z_1)\} d\Lambda_0(s; z_2) \\ &+ \int_0^t \exp\{-\Lambda_0(s; z_2) - \Lambda_*(s; z_1)\}[1 - \exp\{-\Lambda_1(t; z_2) + \Lambda_1(s; z_2)\}] d\Lambda_*(s; z_1), \end{aligned} \tag{S8}$$

because Assumptions (S6) and (S7) essentially have the same meaning with Assumptions (S1) and (S2), respectively (Deng et al., 2024a). The separable direct effect is interpreted as the difference in counterfactual CIFs by manipulating the cause-specific hazards of the terminal event while holding the hazard of the intermediate event unchanged. The separable indirect effect is the difference in counterfactual CIFs by manipulating the hazard of the intermediate event while holding the cause-specific hazards of the terminal event unchanged.

Breum et al. (2024) derived the efficient influence function of the counterfactual CIF and gave an asymptotically efficient estimator in the presence of baseline confounders. To account for time-varying confounders, identification of separable effects requires that the time-varying confounders be also separated, which is referred to as partial isolation (Stensrud et al., 2021). That being said, $Z_1$ directly delivers effect on a set of time-varying confounders $L_1(t)$ and $Z_2$ directly delivers effect on another set of time-varying confounders $L_2(t)$. Estimation can be achieved by discretizing the time periods or applying the continuous version of $g$-formula. Deng et al. (2024a) relaxed the Markovness assumption by considering a semi-Markov case. To relax the dismissible components condition, one may assume a frailty (random effect) following Gamma or lognormal distribution with unknown shape or rate parameters, and the dismissible components condition holds by additionally conditioning on the frailty (Ha et al., 2020). The frailty serves as a time-invariant unmeasured confounder.

# C Identification assumptions with time-varying confounders

Markovness: the hazard of the terminal event only depends on the current status of the intermediate event but not the history, conditional on confounders,

$$\begin{aligned} &P\{d\tilde{N}_2(t;z) = 1 \mid \tilde{N}_2(t^-;z) = 0, \tilde{N}_1(t;z) = n_1, \tilde{N}_1(s;z) = n_0, X = x, \tilde{L}(t) = \tilde{l}(t)\} \\ =\ &P\{d\tilde{N}_2(t;z) = 1 \mid \tilde{N}_2(t^-;z) = 0, \tilde{N}_1(t;z) = n_1, X = x, \tilde{L}(t) = \tilde{l}(t)\},\ s < t. \end{aligned} \tag{S9}$$

Ignorability (exchangeability): the treatment assignment is independent of all potential counting processes, conditional on baseline confounders,

$$Z \perp \{\tilde{N}_1(t;z), \tilde{N}_2(t;z)\} \mid X. \tag{S10}$$

Random censoring: let $d\tilde{N}_c(t;z)$ be the potential counting process of censoring, then it is independent of the potential counting processes of the intermediate and terminal events,

$$\begin{aligned} &P\{d\tilde{N}_c(t;z) = 1 \mid \tilde{N}_c(t^-;z) = 0, \tilde{N}_1(\cdot;z), \tilde{N}_2(\cdot;z), Z = z, X = x, \tilde{L}(t) = \tilde{l}(t)\} \\ =\ &P\{d\tilde{N}_c(t;z) = 1 \mid \tilde{N}_c(t^-;z) = 0, Z = z, X = x, \tilde{L}(t) = \tilde{l}(t)\}. \end{aligned} \tag{S11}$$

Positivity: the supports of confounders overlap and censoring time is large enough,

$$\begin{aligned} &P\{X, \tilde{L}(t)\} > 0 \\ \Rightarrow\ &P\{Z \mid X, \tilde{L}(t)\} > 0, \\ &P\{\tilde{N}_1(t;z) = n_1, \tilde{N}_2(t;z) = 0 \mid X, \tilde{L}(t)\} > 0, \\ \Rightarrow\ &P\{Z = z, \tilde{N}_1(t;z) = n_1, \tilde{N}_2(t;z) = 0, \tilde{N}_c(t;z) = 0 \mid X, \tilde{L}(t)\} > 0. \end{aligned} \tag{S12}$$

Consistency: let $\tilde{T}_1(z)$, $\tilde{T}_2(z)$ and $\tilde{C}(z)$ be the jump times of $\tilde{N}_1(t;z)$, $\tilde{N}_2(t;z)$ and $\tilde{N}_c(t;z)$, let $(T_1, \Delta_1)$, $(T_2, \Delta_2)$ be the pairs of observed event time and censoring indicator, then

$$T_1 = \tilde{T}_1(Z) \wedge \tilde{C}(Z),\ T_2 = \tilde{T}_2(Z) \wedge \tilde{C}(Z),\ \Delta_1 = I\{\tilde{T}_1(Z) \le \tilde{C}(Z)\},\ \Delta_2 = I\{\tilde{T}_2(Z) \le \tilde{C}(Z)\}. \tag{S13}$$

# D Expressions of estimands in the data application

Separable effects framework (conditional on baseline confounders $x$):

$$\begin{aligned} F_{\mathrm{SE}}(t; z_1, z_2, x) = &\int_0^t \exp\{-\Lambda_0(s; z_2, x, 0) - \Lambda_0^*(s; z_1, x) - \Lambda_*(s; z_1, x, 0)\} d\Lambda_0(s; z_2, x, 0) \\ &+ \int_0^t \int_0^u \exp\{-\Lambda_0(s; z_2, x, 0) - \Lambda_0^*(s; z_1, x) - \Lambda_*(s; z_1, x, 0)\} d\Lambda_0^*(s; z_1, x) \\ &\quad \exp\{-\Lambda_0(u; z_2, x, 1) - \Lambda_*(u; z_1, x, 1) + \Lambda_0(s; z_2, x, 1) + \Lambda_*(s; z_1, x, 1)\} d\Lambda_0(u; z_2, x, 0) \\ &+ \int_0^t \int_0^u \exp\{-\Lambda_0(s; z_2, x, 0) - \Lambda_0^*(s; z_1, x) - \Lambda_*(s; z_1, x, 0)\} d\Lambda_*(s; z_1, x, 0) \\ &\quad \exp\{-\Lambda_1(u; z_2, x, 0) - \Lambda_1^*(u; z_1, x) + \Lambda_1(s; z_2, x, 0) + \Lambda_1^*(s; z_1, x)\} d\Lambda_1(u; z_2, x, 0) \\ &+ \int_0^t \int_0^v \int_0^u \exp\{-\Lambda_0(s; z_2, x, 0) - \Lambda_0^*(s; z_1, x) - \Lambda_*(s; z_1, x, 0)\} d\Lambda_0^*(s; z_1, x) \\ &\quad \exp\{-\Lambda_0(u; z_2, x, 1) - \Lambda_*(u; z_1, x, 1) + \Lambda_0(s; z_2, x, 1) + \Lambda_*(s; z_1, x, 1)\} d\Lambda_*(u; z_1, x, 1) \\ &\quad \exp\{-\Lambda_1(v; z_2, x, 1) + \Lambda_1(r; z_2, x, 1)\} d\Lambda_1(v; z_2, x, 1) \\ &+ \int_0^t \int_0^v \int_0^u \exp\{-\Lambda_0(s; z_2, x, 0) - \Lambda_0^*(s; z_1, x) - \Lambda_*(s; z_1, x, 0)\} d\Lambda_*(s; z_1, x, 0) \\ &\quad \exp\{-\Lambda_1(u; z_2, x, 0) - \Lambda_1^*(u; z_1, x) + \Lambda_1(s; z_2, x, 0) + \Lambda_1^*(s; z_1, x)\} d\Lambda_1^*(u; z_1, x) \\ &\quad \exp\{-\Lambda_1(v; z_2, x, 1) + \Lambda_1(u; z_2, x, 1)\} d\Lambda_1(v; z_2, x, 1). \end{aligned}$$

Interventional effects framework (conditional on baseline confounders $x$):

$$F_{\mathrm{IE}}(t; z_1, z_2, x) = \int_0^t \exp\{-\Lambda_0(s; z_2, x, 0) - \Lambda_0^*(s; z_2, x) - \Lambda_*(s; z_1, x)\} d\Lambda_0(s; z_2, x, 0)$$

$$
\begin{aligned}
&+\int_0^t \int_0^u \exp\{-\Lambda_0(s; z_2, x, 0) - \Lambda_0^*(s; z_2, x) - \Lambda_*(s; z_1, x)\} d\Lambda_0^*(s; z_2, x) \\
&\quad \exp\{-\Lambda_0(u; z_2, x, 1) - \Lambda_*(u; z_1, x) + \Lambda_0(s; z_2, x, 1) + \Lambda_*(s; z_1, x)\} d\Lambda_0(u; z_2, x, 0) \\
&+\int_0^t \int_0^u \exp\{-\Lambda_0(s; z_2, x, 0) - \Lambda_0^*(s; z_2, x) - \Lambda_*(s; z_1, x)\} d\Lambda_*(s; z_1, x, 0) \\
&\quad \exp\{-\Lambda_1(u; z_2, x, 0) - \Lambda_1^*(u; z_2, x) + \Lambda_1(s; z_2, x, 0) + \Lambda_1^*(s; z_2, x)\} d\Lambda_1(u; z_2, x, 0) \\
&+\int_0^t \int_0^v \int_0^u \exp\{-\Lambda_0(s; z_2, x, 0) - \Lambda_0^*(s; z_2, x) - \Lambda_*(s; z_1, x)\} d\Lambda_0^*(s; z_2, x) \\
&\quad \exp\{-\Lambda_0(u; z_2, x, 1) - \Lambda_*(u; z_2, x, 1) + \Lambda_0(s; z_2, x, 1) + \Lambda_*(s; z_1, x)\} d\Lambda_*(u; z_1, x) \\
&\quad \exp\{-\Lambda_1(v; z_2, x, 1) + \Lambda_1(r; z_2, x, 1)\} d\Lambda_1(v; z_2, x, 1) \\
&+\int_0^t \int_0^v \int_0^u \exp\{-\Lambda_0(s; z_2, x, 0) - \Lambda_0^*(s; z_2, x) - \Lambda_*(s; z_1, x)\} d\Lambda_*(s; z_1, x) \\
&\quad \exp\{-\Lambda_1(u; z_2, x, 0) - \Lambda_1^*(u; z_2, x) + \Lambda_1(s; z_2, x, 0) + \Lambda_1^*(s; z_2, x)\} d\Lambda_1^*(u; z_1, x) \\
&\quad \exp\{-\Lambda_1(v; z_2, x, 1) + \Lambda_1(u; z_2, x, 1)\} d\Lambda_1(v; z_2, x, 1),
\end{aligned}
$$

where

$$
\begin{aligned}
d\Lambda_*(t; z_1, x) = &\frac{1 - F_{\text{od}}(t; z_1, x) - F_{\text{og}}(t; z_1, x) - F_{\text{or}}(t; z_1, x)}{1 - F_{\text{od}}(t; z_1, x) - F_{\text{ogd}}(t; z_1, x) - F_{\text{or}}(t; z_1, x)} d\Lambda_*(t; z_1, x, 0) \\
&+ \frac{F_{\text{og}}(t; z_1, x) - F_{\text{ogd}}(t; z_1, x)}{1 - F_{\text{od}}(t; z_1, x) - F_{\text{ogd}}(t; z_1, x) - F_{\text{or}}(t; z_1, x)} d\Lambda_*(t; z_1, x, 1),
\end{aligned}
$$

and

$$
\begin{aligned}
F_{\text{od}}(t; z_1, x) &= \int_0^t \exp\{-\Lambda_0(s; z_1, x, 0) - \Lambda_0^*(s; z_1, x) - \Lambda_*(s; z_1, x, 0)\} d\Lambda_0(s; z_1, x, 0), \\
F_{\text{og}}(t; z_1, x) &= \int_0^t \exp\{-\Lambda_0(s; z_1, x, 0) - \Lambda_0^*(s; z_1, x) - \Lambda_*(s; z_1, x, 0)\} d\Lambda_0^*(s; z_1, x), \\
F_{\text{or}}(t; z_1, x) &= \int_0^t \exp\{-\Lambda_0(s; z_1, x, 0) - \Lambda_0^*(s; z_1, x) - \Lambda_*(s; z_1, x, 0)\} d\Lambda_*(s; z_1, x, 0), \\
F_{\text{ogd}}(t; z_1, x) &= \int_0^t \int_0^u \exp\{-\Lambda_0(s; z_1, x, 0) - \Lambda_0^*(s; z_1, x) - \Lambda_*(s; z_1, x, 0)\} d\Lambda_0^*(s; z_1, x) \\
&\quad \exp\{-\Lambda_0(u; z_1, x, 1) - \Lambda_*(u; z_1, x, 1) + \Lambda_0(s; z_1, x, 1) + \Lambda_*(s; z_1, x, 1)\} d\Lambda_0(u; z_1, x, 1).
\end{aligned}
$$

Conditional interventional effects framework (conditional on baseline confounders $x$):

$$
\begin{aligned}
F_{\text{CIE}}(t; z_1, z_2, x) = &\int_0^t \exp\{-\Lambda_0(s; z_2, x, 0) - \Lambda_0^*(s; z_2, x) - \Lambda_*(s; z_1, x, 0)\} d\Lambda_0(s; z_2, x, 0) \\
&+\int_0^t \int_0^u \exp\{-\Lambda_0(s; z_2, x, 0) - \Lambda_0^*(s; z_2, x) - \Lambda_*(s; z_1, x, 0)\} d\Lambda_0^*(s; z_2, x) \\
&\quad \exp\{-\Lambda_0(u; z_2, x, 1) - \Lambda_*(u; z_1, x, 1) + \Lambda_0(s; z_2, x, 1) + \Lambda_*(s; z_1, x, 1)\} d\Lambda_0(u; z_2, x, 0) \\
&+\int_0^t \int_0^u \exp\{-\Lambda_0(s; z_2, x, 0) - \Lambda_0^*(s; z_2, x) - \Lambda_*(s; z_1, x, 0)\} d\Lambda_*(s; z_1, x, 0) \\
&\quad \exp\{-\Lambda_1(u; z_2, x, 0) - \Lambda_1^*(u; z_2, x) + \Lambda_1(s; z_2, x, 0) + \Lambda_1^*(s; z_2, x)\} d\Lambda_1(u; z_2, x, 0) \\
&+\int_0^t \int_0^v \int_0^u \exp\{-\Lambda_0(s; z_2, x, 0) - \Lambda_0^*(s; z_2, x) - \Lambda_*(s; z_1, x, 0)\} d\Lambda_0^*(s; z_2, x) \\
&\quad \exp\{-\Lambda_0(u; z_2, x, 1) - \Lambda_*(u; z_1, x, 1) + \Lambda_0(s; z_2, x, 1) + \Lambda_*(s; z_1, x, 1)\} d\Lambda_*(u; z_1, x, 1) \\
&\quad \exp\{-\Lambda_1(v; z_2, x, 1) + \Lambda_1(r; z_2, x, 1)\} d\Lambda_1(v; z_2, x, 1) \\
&+\int_0^t \int_0^v \int_0^u \exp\{-\Lambda_0(s; z_2, x, 0) - \Lambda_0^*(s; z_2, x) - \Lambda_*(s; z_1, x, 0)\} d\Lambda_*(s; z_1, x, 0)
\end{aligned}
$$

$$\exp\{-\Lambda_1(u; z_2, x, 0) - \Lambda_1^*(u; z_2, x) + \Lambda_1(s; z_2, x, 0) + \Lambda_1^*(s; z_2, x)\} d\Lambda_1^*(u; z_2, x)$$
$$\exp\{-\Lambda_1(v; z_2, x, 1) + \Lambda_1(u; z_2, x, 1)\} d\Lambda_1(v; z_2, x, 1).$$

# E Estimation in the data application

Suppose that the sample includes $n$ independent individuals. Let $X_i$ be the baseline covariates and $Z_i$ be the treatment for the $i$th individual. Let $T_{ig}$, $T_{i\mathrm{r}}$ and $T_{i\mathrm{d}}$ be the times to GVHD, relapse and death (or censoring), and $\Delta_{ig}$, $\Delta_{i\mathrm{r}}$ and $\Delta_{i\mathrm{d}}$ be the corresponding censoring indicators, respectively. The observed data consist of $\{O_i = (X_i, Z_i, T_{ig}, T_{i\mathrm{r}}, T_{i\mathrm{d}}, \Delta_{ig}, \Delta_{ir}, \Delta_{id}) : i = 1, \ldots, n\}$ In nonparametric maximized likelihood estimation (NPMLE), we regard $\Lambda_{j,z}(\cdot)$ as step functions with jumps on event times (Murphy and Van der Vaart, 2000). Let $\lambda_{j,z}(t)$ be the jump size of $\Lambda_{j,z}(\cdot)$ at $t$. The likelihood function is as follows,

$$L = \prod_{z\in\{0,1\}} \prod_{i:Z_i=z} \exp\left\{-\int_0^{T_{ig}} e^{\beta_{3,z}' X_i + \gamma_{3,z} I(t > T_{i\mathrm{r}})} d\Lambda_{3,z}(t)\right\} \left[e^{\beta_{3,z}' X_i + \gamma_{3,z} I(T_{ig} > T_{i\mathrm{r}})} \lambda_{3,z}(T_{ig})\right]^{\Delta_{ig}}$$
$$\exp\left\{-\int_0^{T_{i\mathrm{r}}} e^{\beta_{1,z}' X_i + \eta_{1,z} I(t > T_{ig})} d\Lambda_{1,z}(t)\right\} \left[e^{\beta_{1,z}' X_i + \eta_{1,z} I(T_{i\mathrm{r}} > T_{ig})} \lambda_{1,z}(T_{i\mathrm{r}})\right]^{\Delta_{i\mathrm{r}}}$$
$$\exp\left\{-\int_0^{T_{i\mathrm{d}}} e^{\beta_{2,z}' X_i + \gamma_{2,z} I(t > T_{i\mathrm{r}}) + \eta_{2,z} I(t > T_{ig})} d\Lambda_{2,z}(t)\right\} \left[e^{\beta_{2,z}' X_i + \gamma_{2,z} I(T_{i\mathrm{d}} > T_{i\mathrm{r}}) + \eta_{2,z} I(T_{i\mathrm{d}} > T_{ig})} \lambda_{2,z}(T_{i\mathrm{d}})\right]^{\Delta_{i\mathrm{d}}}.$$

It consists of three independent parts, for each $z \in \{0, 1\}$,

$$L_{3,z} = \prod_{i:Z_i=z} \exp\left\{-\int_0^{T_{ig}} e^{\beta_{3,z}' X_i + \gamma_{3,z} I(t > T_{i\mathrm{r}})} d\Lambda_{3,z}(t)\right\} \left[e^{\beta_{3,z}' X_i + \gamma_{3,z} I(T_{ig} > T_{i\mathrm{r}})} \lambda_{3,z}(T_{ig})\right]^{\Delta_{ig}}$$
$$L_{1,z} = \prod_{i:Z_i=z} \exp\left\{-\int_0^{T_{i\mathrm{r}}} e^{\beta_{1,z}' X_i + \eta_{1,z} I(t > T_{ig})} d\Lambda_{1,z}(t)\right\} \left[e^{\beta_{1,z}' X_i + \eta_{1,z} I(T_{i\mathrm{r}} > T_{ig})} \lambda_{1,z}(T_{i\mathrm{r}})\right]^{\Delta_{i\mathrm{r}}}$$
$$L_{2,z} = \prod_{i:Z_i=z} \exp\left\{-\int_0^{T_{i\mathrm{d}}} e^{\beta_{2,z}' X_i + \gamma_{2,z} I(t > T_{i\mathrm{r}}) + \eta_{2,z} I(t > T_{ig})} d\Lambda_{2,z}(t)\right\} \left[e^{\beta_{2,z}' X_i + \gamma_{2,z} I(T_{i\mathrm{d}} > T_{i\mathrm{r}}) + \eta_{2,z} I(T_{i\mathrm{d}} > T_{ig})} \lambda_{2,z}(T_{i\mathrm{d}})\right]^{\Delta_{i\mathrm{d}}}.$$

The parameters $\beta_{j,z}$, $\eta_{j,z}$ and $\gamma_{j,z}$ are estimated by solving the score function with respect to these parameters,

$$0 = \sum_{i:Z_i=z} \Delta_{ig} \left[X_i - \frac{\sum_{k:Z_k=z} I(T_{k\mathrm{g}} \ge T_{i\mathrm{g}}) \exp\{\beta_{3,z}' X_k + \gamma_{3,z} I(T_{i\mathrm{g}} > T_{k\mathrm{r}})\} X_k}{\sum_{k:Z_k=z} I(T_{k\mathrm{g}} \ge T_{i\mathrm{g}}) \exp\{\beta_{3,z}' X_k + \gamma_{3,z} I(T_{i\mathrm{g}} > T_{k\mathrm{r}})}\right],$$
$$0 = \sum_{i:Z_i=z} \Delta_{i\mathrm{r}} \left[X_i - \frac{\sum_{k:Z_k=z} I(T_{k\mathrm{r}} \ge T_{i\mathrm{r}}) \exp\{\beta_{1,z}' X_k + \eta_{1,z} I(T_{i\mathrm{r}} > T_{kg})\} X_k}{\sum_{k:Z_k=z} I(T_{k\mathrm{r}} \ge T_{i\mathrm{r}}) \exp\{\beta_{1,z}' X_k + \eta_{1,z} I(T_{i\mathrm{r}} > T_{kg})}\right],$$
$$0 = \sum_{i:Z_i=z} \Delta_{i\mathrm{d}} \left[X_i - \frac{\sum_{k:Z_k=z} I(T_{k\mathrm{d}} \ge T_{i\mathrm{d}}) \exp\{\beta_{2,z}' X_k + \gamma_{2,z} I(T_{i\mathrm{d}} > T_{k\mathrm{r}}) + \eta_{2,z} I(T_{i\mathrm{d}} > T_{kg})\} X_k}{\sum_{k:Z_k=z} I(T_{k\mathrm{d}} \ge T_{i\mathrm{d}}) \exp\{\beta_{2,z}' X_k + \gamma_{2,z} I(T_{i\mathrm{d}} > T_{k\mathrm{r}}) + \eta_{2,z} I(T_{i\mathrm{d}} > T_{kg})}\right],$$
$$0 = \sum_{i:Z_i=z} \Delta_{ig} \left[I(T_{ig} > T_{i\mathrm{r}}) - \frac{\sum_{k:Z_k=z} I(T_{k\mathrm{g}} \ge T_{i\mathrm{g}} > T_{k\mathrm{r}}) \exp\{\beta_{3,z}' X_k + \gamma_{3,z} I(T_{i\mathrm{g}} > T_{k\mathrm{r}})\}}{\sum_{k:Z_k=z} I(T_{k\mathrm{g}} \ge T_{i\mathrm{g}}) \exp\{\beta_{3,z}' X_k + \gamma_{3,z} I(T_{i\mathrm{g}} > T_{k\mathrm{r}})}\right],$$
$$0 = \sum_{i:Z_i=z} \Delta_{i\mathrm{r}} \left[I(T_{i\mathrm{r}} > T_{ig}) - \frac{\sum_{k:Z_k=z} I(T_{k\mathrm{r}} \ge T_{i\mathrm{r}} > T_{kg}) \exp\{\beta_{1,z}' X_k + \eta_{1,z} I(T_{i\mathrm{r}} > T_{kg})\}}{\sum_{k:Z_k=z} I(T_{k\mathrm{r}} \ge T_{i\mathrm{r}}) \exp\{\beta_{1,z}' X_k + \eta_{1,z} I(T_{i\mathrm{r}} > T_{kg})}\right],$$
$$0 = \sum_{i:Z_i=z} \Delta_{i\mathrm{d}} \left[I(T_{i\mathrm{d}} > T_{i\mathrm{r}}) - \frac{\sum_{k:Z_k=z} I(T_{k\mathrm{d}} \ge T_{i\mathrm{d}} > T_{k\mathrm{r}}) \exp\{\beta_{2,z}' X_k + \eta_{2,z} I(T_{i\mathrm{d}} > T_{k\mathrm{r}}) + \gamma_{2,z} I(T_{i\mathrm{d}} > T_{kg})\}}{\sum_{k:Z_k=z} I(T_{k\mathrm{d}} \ge T_{i\mathrm{d}}) \exp\{\beta_{2,z}' X_k + \eta_{2,z} I(T_{i\mathrm{d}} > T_{k\mathrm{r}}) + \gamma_{2,z} I(T_{i\mathrm{d}} > T_{kg})\}}\right],$$
$$0 = \sum_{i:Z_i=z} \Delta_{i\mathrm{d}} \left[I(T_{i\mathrm{d}} > T_{ig}) - \frac{\sum_{k:Z_k=z} I(T_{k\mathrm{d}} \ge T_{i\mathrm{d}} > T_{kg}) \exp\{\beta_{2,z}' X_k + \eta_{2,z} I(T_{i\mathrm{d}} > T_{k\mathrm{r}}) + \gamma_{2,z} I(T_{i\mathrm{d}} > T_{kg})\}}{\sum_{k:Z_k=z} I(T_{k\mathrm{d}} \ge T_{i\mathrm{d}}) \exp\{\beta_{2,z}' X_k + \eta_{2,z} I(T_{i\mathrm{d}} > T_{k\mathrm{r}}) + \gamma_{2,z} I(T_{i\mathrm{d}} > T_{kg})\}}\right],$$

denoted by $\hat{\beta}_{j,z}$, $\hat{\eta}_{j,z}$ and $\hat{\gamma}_{j,z}$, respectively, and the hazards are estimated by

$$\hat{\lambda}_{3,z}(t) = \frac{\sum_{i:Z_i=z} \Delta_{ig} I(T_{ig} = t)}{\sum_{i:Z_i=z} I(T_{ig} \geq t) \exp\{\hat{\beta}'_{3,z} X_i + \hat{\gamma}_{3,z} I(t > T_{ir})\}},$$
$$\hat{\lambda}_{1,z}(t) = \frac{\sum_{i:Z_i=z} \Delta_{ir} I(T_{ir} = t)}{\sum_{i:Z_i=z} I(T_{ir} \geq t) \exp\{\hat{\beta}'_{1,z} X_i + \hat{\eta}_{1,z} I(t > T_{ig})\}},$$
$$\hat{\lambda}_{2,z}(t) = \frac{\sum_{i:Z_i=z} \Delta_{id} I(T_{id} = t)}{\sum_{i:Z_i=z} I(T_{id} \geq t) \exp\{\hat{\beta}'_{2,z} X_i + \hat{\gamma}_{2,z} I(t > T_{ir}) + \hat{\eta}_{2,z} I(t > T_{ig})\}}.$$

# F Frailty modeling in the data application

We assume the following proportional hazards models,

$$d\Lambda_*(t; z, x, l, b) = d\Lambda_{1,z}(t) \exp(\beta'_{1,z} x + \gamma_{1,z} l + \alpha_z b),$$
$$d\Lambda_{n_1}(t; z, x, l, b) = d\Lambda_{2,z}(t) \exp(\beta'_{2,z} x + \gamma_{2,z} l + \eta_{2,z} n_1 + \alpha_z b),$$
$$d\Lambda^*_{n_1}(t; z, x, b) = d\Lambda_{3,z}(t) \exp(\beta'_{3,z} x + \eta_{3,z} n_1 + \alpha_z b),$$

where $b \sim N(0, 1)$ is a frailty and $\alpha_z > 0$. We assume that sequential ignorability (or dismissible components condition) holds conditional on the baseline confounders $x$ and frailty $b$. Let $F(t; z_1, z_2, x, b)$ the counterfactual CIF of the terminal event conditional on baseline confounders $x$ and frailty $b$, then the population-level counterfactual CIF

$$F(t; z_1, z_2) = \int_{\mathcal{X}} \int_{-\infty}^{+\infty} F(t; z_1, z_2, x, b) \phi(b) db dP(x),$$

where $\phi(b) = (2\pi)^{-1/2} \exp(-b^2/2)$ is the density function of $b$.

We use the EM algorithm to estimate the parameters. Let $f(O, b; \theta)$ be the density function of complete data (including observed data $O$ and missing data $b$) evaluated at the parameter value $\theta \in \Theta$ for a single individual. In the E step, we calculate the expectation of any function of complete data $Q(O_i, b_i)$ conditional on observed data and current parameter $\hat{\theta}$,

$$\hat{E}\{Q(O_i, b_i)\} = \frac{\int_{-\infty}^{+\infty} f(O_i, b; \hat{\theta}) Q(O_i, b) \phi(b) db}{\int_{-\infty}^{+\infty} f(O_i, b; \hat{\theta}) \phi(b) db}.$$

The numerical integral is evaluated by Gaussian quadrature. In the M step, we update parameter $\hat{\theta}$. Specifically,

$$\hat{\lambda}_{3,z}(t) = \frac{\sum_{i:Z_i=z} \Delta_{ig} I(T_{ig} = t)}{\sum_{i:Z_i=z} I(T_{ig} \geq t) \hat{E}[\exp\{\hat{\beta}'_{3,z} X_i + \hat{\gamma}_{3,z} I(t > T_{ir}) + \hat{\alpha}_z b_i\}]},$$
$$\hat{\lambda}_{1,z}(t) = \frac{\sum_{i:Z_i=z} \Delta_{ir} I(T_{ir} = t)}{\sum_{i:Z_i=z} I(T_{ir} \geq t) \hat{E}[\exp\{\hat{\beta}'_{1,z} X_i + \hat{\eta}_{1,z} I(t > T_{ig}) + \hat{\alpha}_z b_i\}]},$$
$$\hat{\lambda}_{2,z}(t) = \frac{\sum_{i:Z_i=z} \Delta_{id} I(T_{id} = t)}{\sum_{i:Z_i=z} I(T_{id} \geq t) \hat{E}[\exp\{\hat{\beta}'_{2,z} X_i + \hat{\gamma}_{2,z} I(t > T_{ir}) + \eta_{2,z} I(t > T_{ig}) + \hat{\alpha}_z b_i\}]}.$$

By regarding $b_{iz} = \alpha_z b_i$ instead of $b_i$ as missing data,

$$\hat{\alpha}_z^2 = |\{i : Z_i = z\}|^{-1} \sum_{i:Z_i=z} \hat{E}(b_{iz}^2).$$

The effect of the frailty is estimated at $\hat{\alpha}_1 = 0.31$ in the Haplo-SCT group and $\hat{\alpha}_0 = 0.13$ in the MSDT group. The frailty effects are small, indicating that the correlation between the hazards of GVHD, relapse and death is weak. This confirms the robustness of the substantial conclusion in the main text. In addition, we find that relapse increases the hazard of death by about 28 times in the Haplo-SCT group. GVHD reduces the hazard of relapse by about 22% and increases the hazard of death by about 5.5%. The graft-versus-leukemia effect is strong and beneficial for overall survival. However, the graft-versus-leukemia

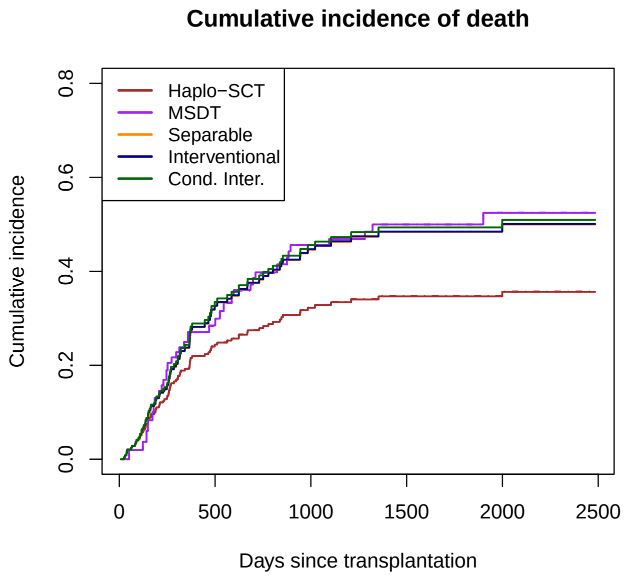


Figure S1: Estimated cumulative incidence functions of death associated with MSDT, Haplo-SCT and in the counterfactual worlds (separable effects, interventional effects and conditional interventional effects) using frailty modeling. The solid lines are $F(t; z)$ and the dashed lines are $F_{\mathrm{IE}}(t; z, z)$ for Haplo-SCT and MSDT: they are very close.

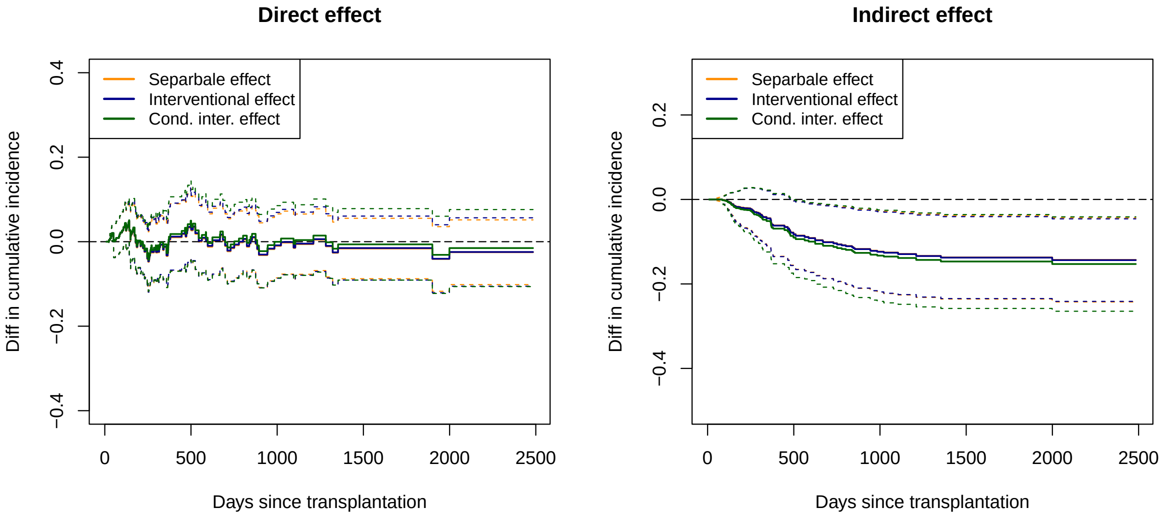


Figure S2: Estimated direct and indirect effects for different estimands (separable effects, interventional effects and conditional interventional effects) using frailty modeling. Confidence intervals are obtained by bootstrap.

effect does not exist in the MSDT group ($\hat{\gamma}_{1,1} > 0$). Due to the limited sample size, the standard errors of the estimates are large.

Figure S1 shows the estimated CIFs of death associated with MSDT, Haplo-SCT and in the counterfactual worlds in solid lines. Specially for the interventional approach, we display the counterfactual CIFs (not equal to potential CIFs) under MSDT and Haplo-SCT in dashed lines. Figure S2 shows the estimated direct and indirect effects. The three estimators show similar patterns in this study, and are vert similar to the estimates in the main text.

# References


Breum, M. S., Munch, A., Gerds, T. A., and Martinussen, T. (2024). Estimation of separable direct and indirect effects in a continuous-time illness-death model. *Lifetime Data Analysis*, 30(1):143–180.

Deng, Y., Wang, Y., Zhan, X., and Zhou, X.-H. (2024a). Separable pathway effects of semi-competing risks using multi-state models. *arXiv preprint arXiv:2306.15947v2*.

Deng, Y., Wang, Y., and Zhou, X.-H. (2024b). Direct and indirect treatment effects in the presence of semicompeting risks. *Biometrics*, 80(2):ujae032.

Ha, I. D., Xiang, L., Peng, M., Jeong, J.-H., and Lee, Y. (2020). Frailty modelling approaches for semi-competing risks data. *Lifetime Data Analysis*, 26:109–133.

Huang, Y.-T. (2021). Causal mediation of semicompeting risks. *Biometrics*, 77(4):1143–1154.

Murphy, S. A. and Van der Vaart, A. W. (2000). On profile likelihood. *Journal of the American Statistical Association*, 95(450):449–465.

Robins, J. M., Richardson, T. S., and Shpitser, I. (2022). An interventionist approach to mediation analysis. In *Probabilistic and causal inference: the works of Judea Pearl*, pages 713–764.

Stensrud, M. J., Hernán, M. A., Tchetgen Tchetgen, E. J., Robins, J. M., Didelez, V., and Young, J. G. (2021). A generalized theory of separable effects in competing event settings. *Lifetime Data Analysis*, 27(4):588–631.
